# Supplementary material for: Sweep Complexity Revisited
Source: arXiv:2308.06683 source file (2023-08-13)
Supplement: Supplementary file 1 [file rev_appendix.tex]

\newpage
\section{Appendix}\label{Sec:appendix}

\subsection{Counting the sweep complexity of rejected words}
We defined the sweep complexity of a machine as the maximum number of sweeps over all \emph{accepted} words of length $n$. One could also take into account the sweep count of rejected words. However, this would allow a trick in a sense to `artificially' increase the sweep complexity of machines with complexity $o(n)$ without affecting regularity. Let $A$ be a machine accepting a regular language and $B$ a non-regular language with sweep complexities $f(n)$ and $g(n)$, respectively, such that $f(n)\in o(g(n))$. The we can easily construct a ROWJFA accepting $aL(A)$ with sweep complexity $g(n)$ by adding a new initial state from which reading $a$ takes us to the initial state of $A$ while reading $b$ takes us to the initial state of $B$. We set all states of $B$ non-final and this way we get that on inputs starting with $b$ the machine performs $B$'s computations but never accepts anything. Moreover, $aL(A)$ is regular if and only if $L(A)$ was.

\begin{figure}
    \centering
    \input{fig/appendrejectcompl}
    \caption{Artificially increasing the complexity by adding non-functional states to the automaton.}
    \label{fig:my_label}
\end{figure}
